# Supplementary material for: Search for Light Dark Matter-Electron Scatterings in the PandaX-II Experiment
Source: arXiv:2101.07479 ancillary file (2021-05-07)
Supplement: Supplementary file 1 [file Supplementary_Material.pdf]

# SUPPLEMENTARY MATERIALS

## Time Isolation Cut

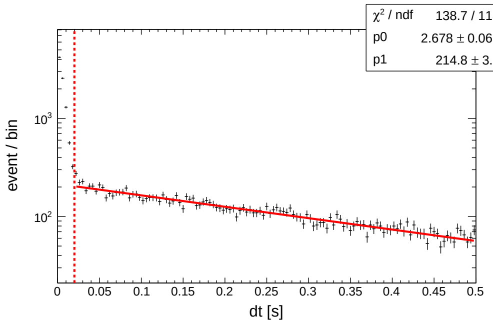


FIG. 1. Time-to-previous event distribution for the US2s within 50 to 200 PE (fiducial cut applied)

, with the 0.02 s isolation cut indicated. No time correlation of the candidate US2s is found to the previous energetic events. The residual slope is consistent with a trigger rate of ~3 Hz.

The isolation cut of 0.02 s is set to remove correlated single electron trains happening after large signals. The distribution is shown in Fig. 1. The distribution after 0.02 s is consistent with a Poisson distributed event rate of ~3 Hz. For the remaining candidates of US2s, we didn't find an obvious correlation between them and previous events.

## Data Quality Cuts

Run 11 tritium calibration data and dark matter run data, with $S2$ charge-dependent cuts (red curves) overlaid, are shown in Fig.4. All three cuts, including the full-width-10%-maxima, the rising edge (defined as the ratio of the charge in the first 1 $\mu$s to the total), and the top/bottom charge ratio of the US2s, are developed based on the distribution of the tritium calibration data.

## Fiducial Volume

Compared to Ref. [1], events in this analysis are selected with a more conservative radial cut so events within 15 cm from the wall are removed to avoid un-paired field cage surface events, leading to a 117.0 ± 6.6 kg fiducial mass of liquid xenon. The uncertainty is dominated by the 4.2 mm radial position resolution, estimated using different reconstruction algorithms. For the remaining candidate, the horizontal distribution within

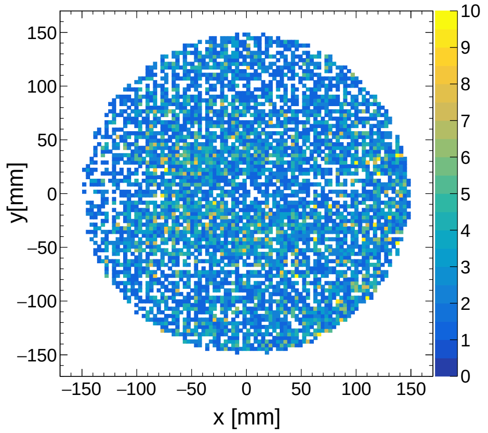


FIG. 2. Spatial distribution of candidates in the ROI

the fiducial volume is mostly uniform, as shown in Fig. 2.

## Details on Trigger Efficiency Uncertainty

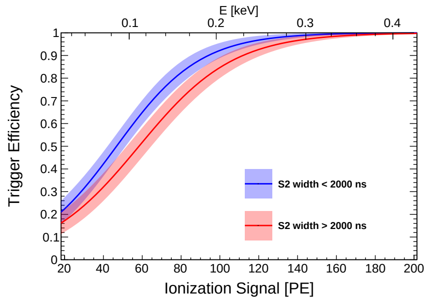


FIG. 3. The trigger efficiencies vs. S2 with two groups of S2 widths

For $S2$s considered in our ROI, the width is approximately in between 1000 ns to 3000 ns (see Fig. 5). We take the data from Ref. [2], and separate them into two groups, below 2000 ns and above 2000 ns. Trigger efficiencies for these two groups are plotted Fig. 3, with the difference less than ±12% in the ROI.

In regarding to whether the trigger may have a drift time dependence, we also show paired $S1 + S2$ events for $^{241}$Am-Be in Fig. 5 (statistics for paired $S1 + S2$ tritium events are very small in the low energy region) for $S2$ within 50 and 75 PE. The effect of the widening of $S2$ vs. longer drift time is very negligible at this low S2 range.

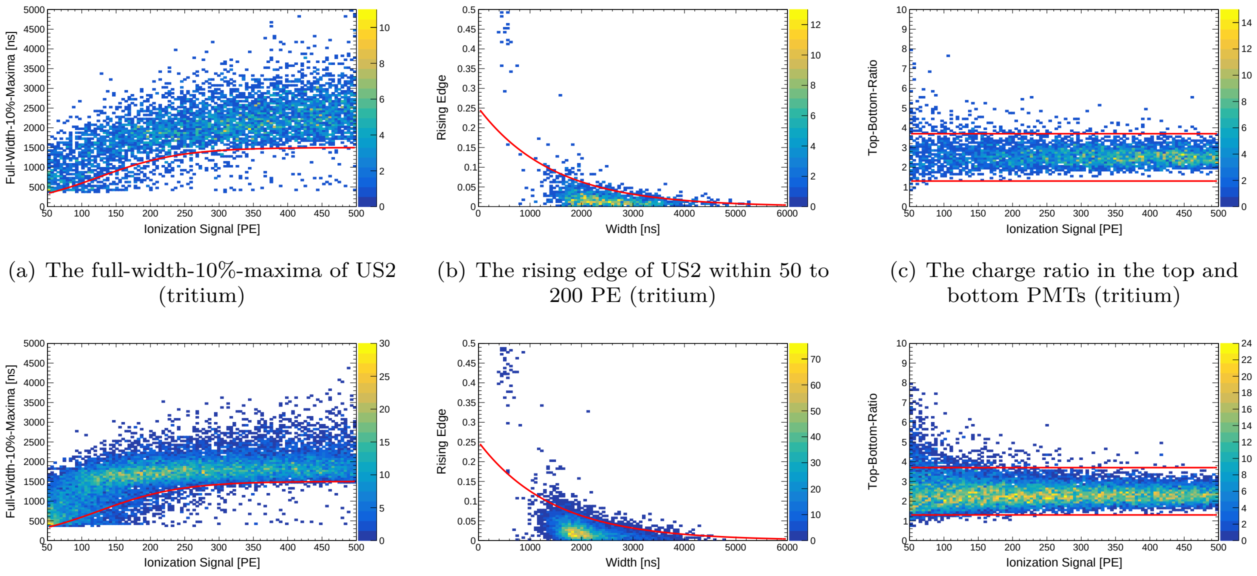


(a) The full-width-10%-maxima of US2 (tritium)

(b) The rising edge of US2 within 50 to 200 PE (tritium)

(c) The charge ratio in the top and bottom PMTs (tritium)

(d) The full-width-10%-maxima of US2 (dark matter run)

(e) The rising edge of US2 within 50 to 200 PE (dark matter run)

(f) The charge ratio in the top and bottom PMTs (dark matter run)

FIG. 4. Run 11 tritium calibration data and dark matter run data, and the charge-dependent cuts (red curves) for the width, rising edge, and the top/bottom ratio of US2. Note that the ROI for the dark matter search is between 50 and 75 PE.

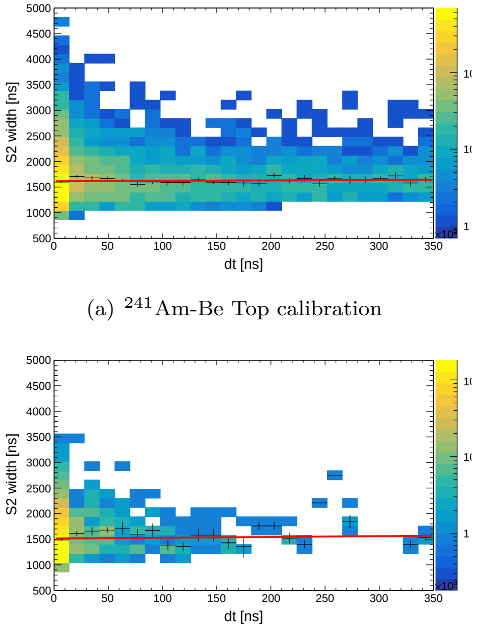


(a) $^{241}$Am-Be Top calibration

(b) $^{241}$Am-Be Bottom calibration

FIG. 5. Drift time vs. widths of $S2$s from $^{241}$Am-Be calibration events with $S2$ in the range of 50−75 PE (ROI). Red lines are linear fits.

### Details on Uncertainties of Data Quality Cut Efficiency

*Effect of non-source events in calibration data*

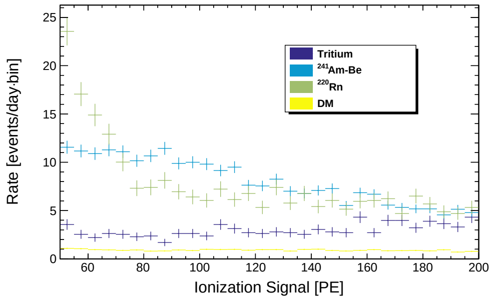


FIG. 6. Event rates of calibration (tritium, $^{220}$Rn and $^{241}$Am-Be) and DM runs in Run 11.

In all calibration runs, the event introduced by the calibration sources dominate over the non-source "background" in the dark matter data (see Fig. 6). Under the existence of background, the measured efficiency can be written as

$$\epsilon = \frac{\epsilon_1 N_1 + \epsilon_2 N_2}{N_1 + N_2}\,, \qquad (1)$$

in which $\epsilon$ is our estimated cut efficiency, and $\epsilon_1$ ($\epsilon_2$) and $N_1$ ($N_2$) are the efficiency and number of events for

the source (non-source) data, respectively. If we take Run 11 tritium data (worst case in terms of S/B ratio) as an example, the source/non-source ratio in the ROI is roughly 9/5. By varying $\epsilon_2$ between 0.5 and 0.75, twice of the total range between the tritium and $^{241}$Am-Be data sets in the ROI (Fig. 2 of the paper), the true $\epsilon_1$ changes within $\pm 10.0\%$ (fractional) under the same $\epsilon$. If one were to apply an $\epsilon_2$ evaluated using 10% DM data (a small fraction to avoid circular argument), the variation in $\epsilon_1$ is even less. Therefore, we keep the same nominal (measured) efficiency from tritium calibration data, but assign $\pm 10\%$ as a systematic uncertainty due to the existence of non-source events.

*Shape dependence of data selection efficiency*

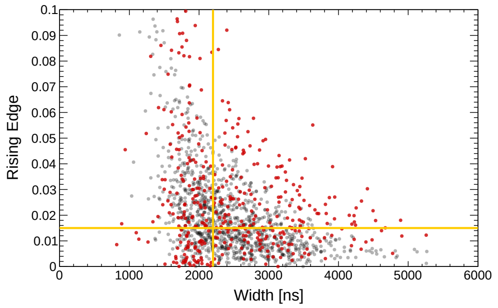


FIG. 7. The distribution of the rising edge vs. width for Run 11 tritium US2 events within 50 to 200 PE. The width cut of 2200 ns and the rising edge cut of 0.015 are indicated as the vertical and horizontal solid orange lines. The red/black dots represent the removed/survived data with the combined $S2$ width, rising edge, and the top/bottom ratio cuts.

To study the waveform shape dependence of the selection efficiency, in Fig. 7, we show the distribution of tritium events in rising edge vs. width. We separate the data into two halves, either by the rising edge (horizontal line) or by the width (vertical line). These abrupt partitions should capture potential systematics either due to electron cloud diffusion or electroluminescence non-uniformity. The resulting selection efficiencies are shown in Fig. 8, indicating the level of waveform shape dependence.

To further reinforce this point, we also show the efficiencies of $^{241}$Am-Be calibration runs (source located in the top and bottom calibration tubes), as well as the diffusive $^{220}$Rn efficiency. The RMS of the seven aforementioned efficiency curves is 9.2% (fractional) in the ROI, which serves as an estimate of the systematic uncertainty in data selection cuts.

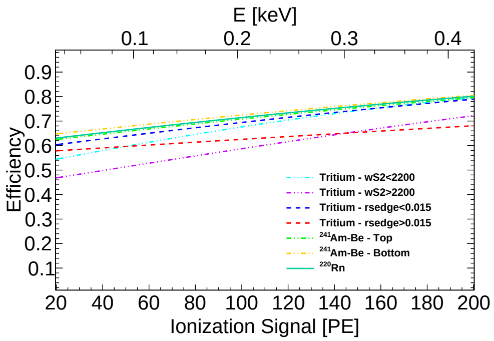


FIG. 8. Cut efficiencies vs. $S2$ charge in different $S2$ width and rising edge partitions for tritium events, and for $^{241}$Am-Be top or bottom, and the $^{220}$Rn events.

*Data and MC Comparison for Tritium Events*

The data and MC comparison for the tritium events are shown in Fig. 9, (a): paired S1+S2 which set the normalization, (b): US2s. One sees that the measured US2 rate in the tritium data is on average nine times larger than the MC expectation in the ROI, despite a good match at higher $S2$. As shown in Fig 6, the events introduced by the tritium source in calibration run dominate over the non-source events in the dark matter data. Since such excess is clearly related to the tritium injection, it cannot be produced by dark matter.

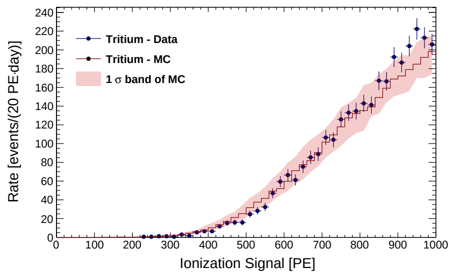


(a) MC vs. Paired S1+S2 Data

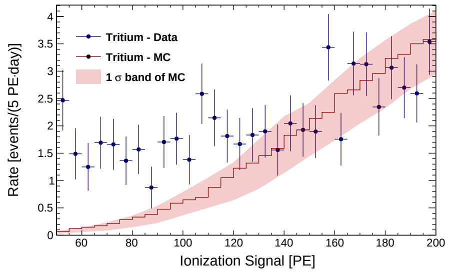


(b) MC vs. US2 Data

FIG. 9. Predicted vs. observed S2 distributions for Run 11 tritium calibration events.

### Uncertainty of $S2$ Identification

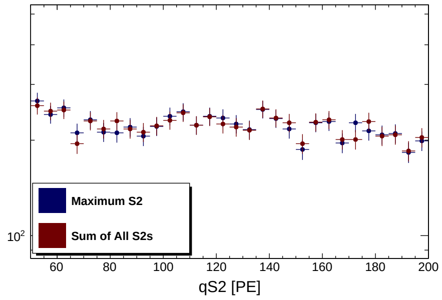


FIG. 10. Spectral comparison between sum of all S2s detected in a waveform, and the maximum S2.

The total charge of all $S2$s detected in a given waveform (if they are broken up into several) and the maximum $S2$ is shown in Fig.10 and little spectrum change is observed. At this low energy, potentially a single S2 could be recognized as multiple single-electron-S2s. The efficiency is estimated to be $100^{+1.5}_{-1.5}\%$, based on the change of event rate in the ROI using the maximum S2 or the sum of S2s.


[1] Q. Wang *et al.* (PandaX-II), Chin. Phys. C **44**, 125001 (2020).

[2] Q. Wu *et al.*, JINST **12** (08), T08004.
